# Supplementary material for: Investigating the 'Autoencoder Behavior' in Speech Self-Supervised Models: a focus on HuBERT's Pretraining
Source: arXiv:2405.08402 source file (2024-05-14)
Supplement: Supplementary file 1 [file appendix.tex]

\section{Appendix}
\begin{figure*}[h!]
    \centering
    \begin{minipage}{0.4\linewidth}
        \caption*{\tiny{CCA-AGWE} }
        \vspace{-0.4cm}
        \includegraphics[width=\textwidth]{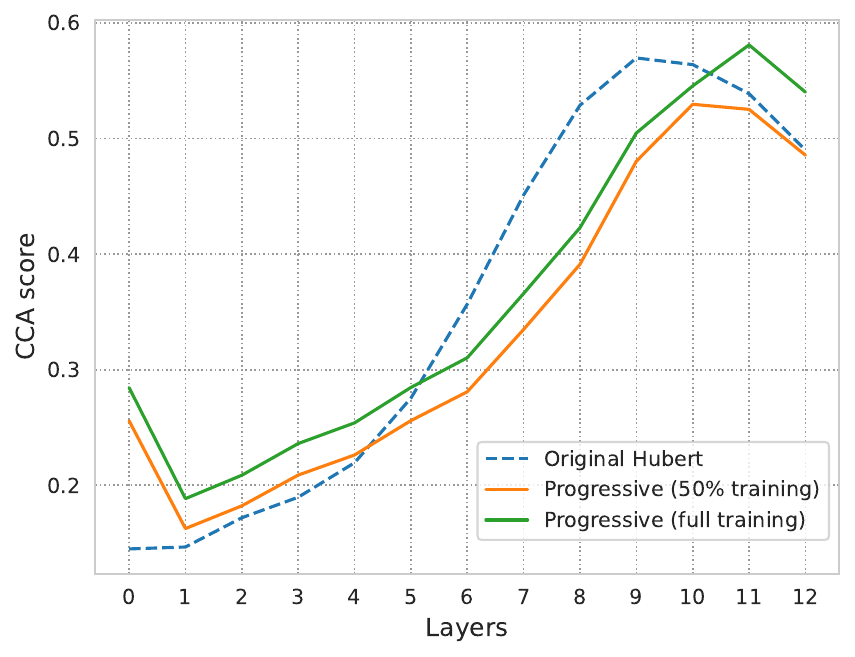}
    \end{minipage}
    \centering
    \begin{minipage}{0.4\linewidth}
        \caption*{\tiny{CCA-GloVe} }
        \vspace{-0.4cm}
        \includegraphics[width=\textwidth]{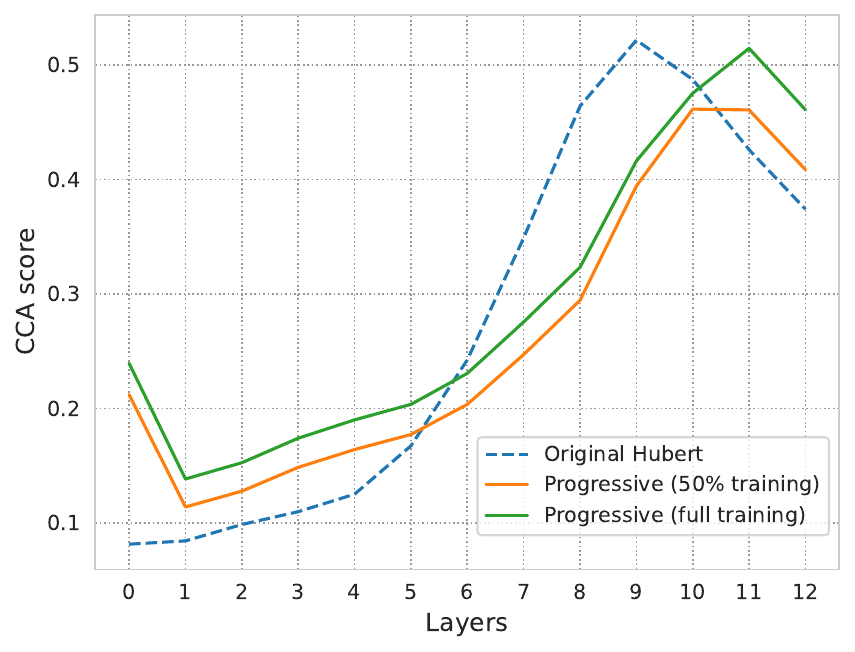}
    \end{minipage}
    \caption{Layerwise AGWE and GloVe CCA similarites for Original and Progressive approaches.}
    \label{fig:agwe}
\end{figure*}
\subsection{Total computational budget}
This paper required around 10,000 GPU hours, with a non negligible part dedicated to failures in the replication of the official HuBERT results.

\subsection{Implementation details}
We train the HuBERT Base model, that is denoted as \textit{Original} in this paper. We base our implementation on \href{https://github.com/pytorch/audio/tree/main/examples/hubert}{torchaudio} and use the hyperparameters proposed in the Original article~\cite{hsu2021hubert}, except for minor changes detailed below.

In order to compute the discrete units clusters on the whole dataset without using a large CPU RAM, we modify the clustering step by implementing real minibatch-kmeans (with partial fitting for each minibatch).
The pretraining step uses only four 3090 GPUs and therefore accumulate gradients to keep the same virtual batch size. Other hyperparameters are kept unchanged. 
Finetuning on the LibriLight-10h~\cite{kahn2020libri} and \href{https://github.com/ankitapasad/layerwise-analysis}{layerwise evaluation} are performed following the official repositories.

For the Uniform and Progressive strategies, we use 100 clusters for all iterations, while for Progressive+Cluster, we linearly increase the number of clusters from 100 at the first iteration to 500 at the last. 

The gap between our implementation and the official results may be due to the usage of less GPUs during pretraining. Indeed, even with gradient accumulation, the virtual batch size is not strictly equivalent, because modules such as Batch Normalization are computed during the forward pass.

\subsection{Layerwise Analysis through training for different models}
We propose in Figure~\ref{fig:layerwise} a detailed layerwise analysis during the training of HuBERT and Wav2vec2. It shows further illustrations of the "autoencoder" behavior, which is alleviated by the second iteration of HuBERT. 
Layerwise analysis is computing the similarity between the model embeddings and Acoustically Grounded Word Embeddings~\cite{settle2019acoustically}, Phone (one-hot of phone labels), Word (one-hot of word label), or Wrt Layer0 (embedding of the layer 0).

\subsection{Convergence failures}
We also analyse other strategies, which does not manage to achieve convergence.
\textbf{Warm start from the previous iteration checkpoint}
We propose to modify the \textit{Progressive} approach by reusing at every iteration the checkpoint of the previous one. This results in a surprising behaviour, where the pretraining loss decreases strongly during few minibatch steps and then just diverge to constant values. An explanation may be that the current supervision is computed from the very model embeddings and that collapsing is therefore easy to fulfill.

\textbf{Impact of the iteration size}
The minimal size we observe for one iteration was 12000 mini-batch steps.

\textbf{Decreasing the iteration size}
We did a single \textit{Progressive} training run by linearly decreasing the iteration sizes. We observe convergence on the first iteration, but the model diverged during iteration 6.

\textbf{Layerwise AGWE and GloVE}

As a supplementary analysis of word-level representation, we also observe in Figure~\ref{fig:agwe} the model behaviour for AGWE and GloVe similarites, leading to the same conclusions than for Word similarity presented in the Results of the paper.

\begin{figure*}
    \centering
    \begin{minipage}{0.32\linewidth}
        \caption*{\tiny{HuBERT First Iteration - AGWE} }
        \includegraphics[width=\textwidth]{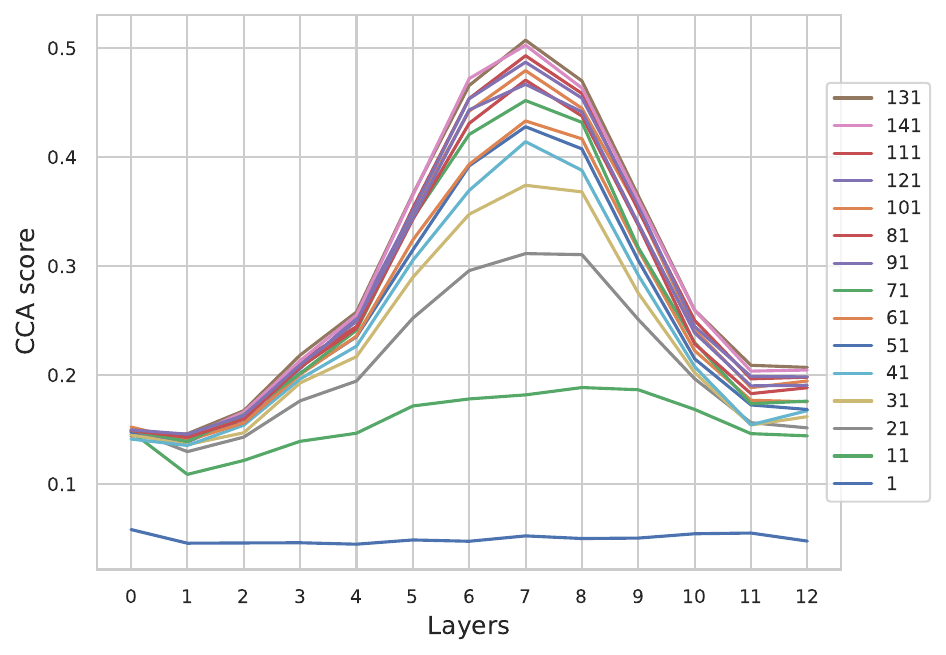} 
        
    \end{minipage}
    \centering
    \begin{minipage}{0.32\linewidth}
        \caption*{\tiny{HuBERT Second Iteration - AGWE} }
        \includegraphics[width=\textwidth]{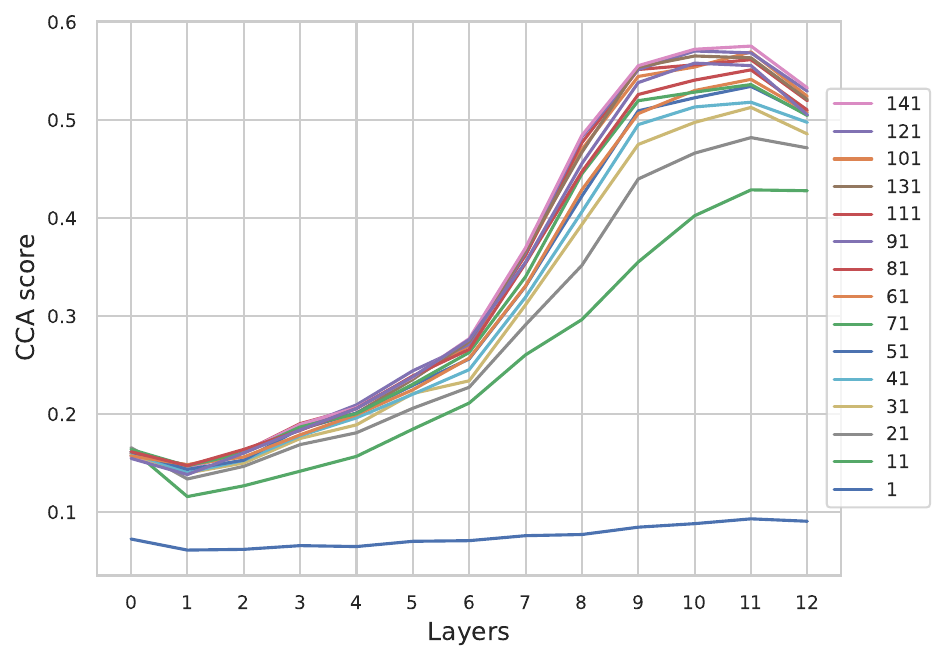}
        
    \end{minipage}
    \centering
    \begin{minipage}{0.32\linewidth}
        \caption*{\tiny{Wav2vec2.0 - AGWE} }
        \includegraphics[width=\textwidth]{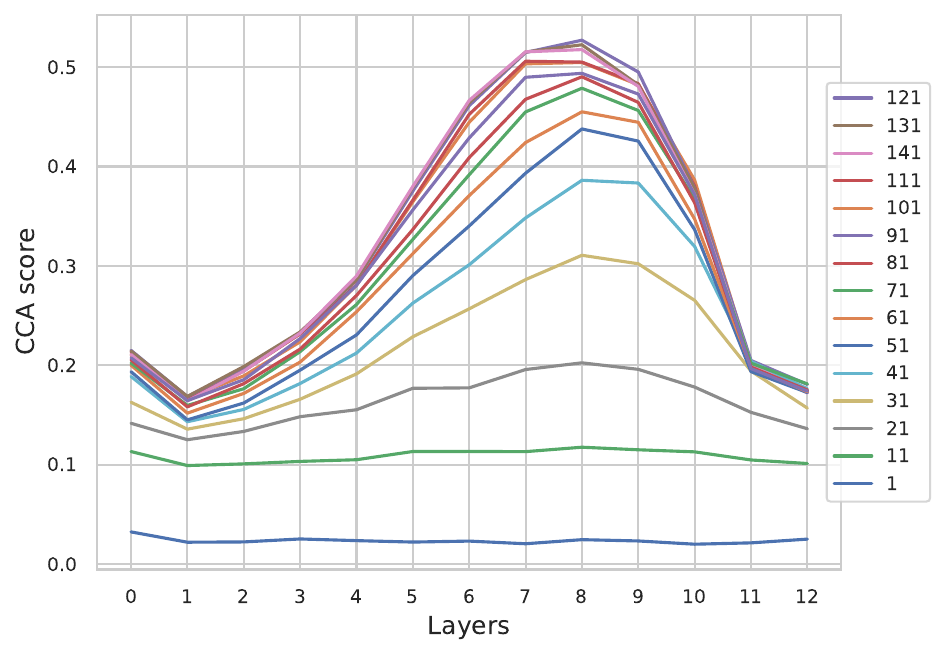}
        
    \end{minipage}
     \centering
    \begin{minipage}{0.32\linewidth}
        \caption*{\tiny{HuBERT First Iteration - Word} }
        \includegraphics[width=\textwidth]{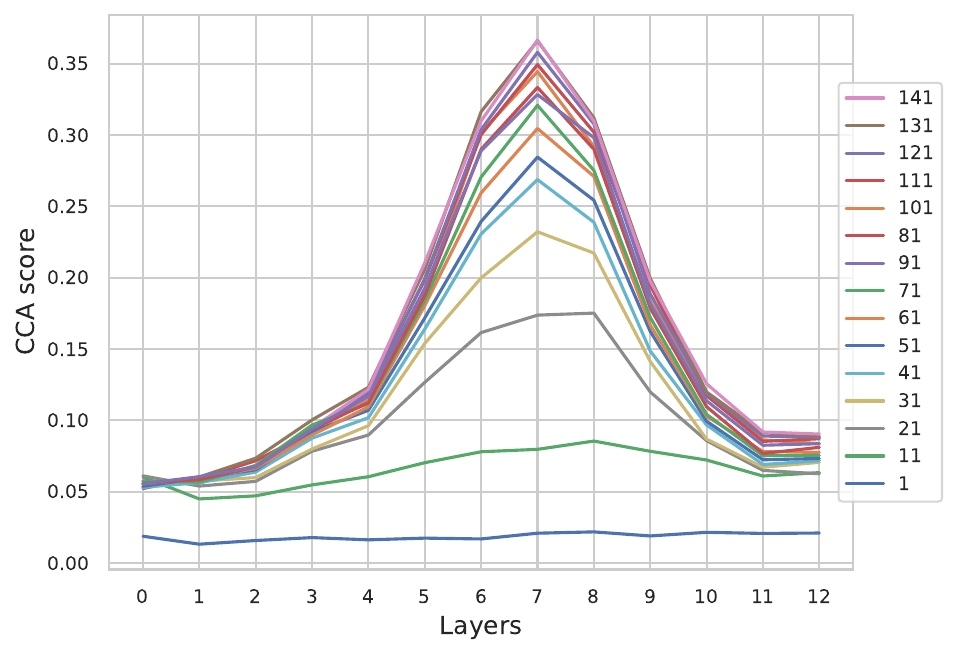} 
        
    \end{minipage}
    \centering
    \begin{minipage}{0.32\linewidth}
        \caption*{\tiny{HuBERT Second Iteration - Word} }
        \includegraphics[width=\textwidth]{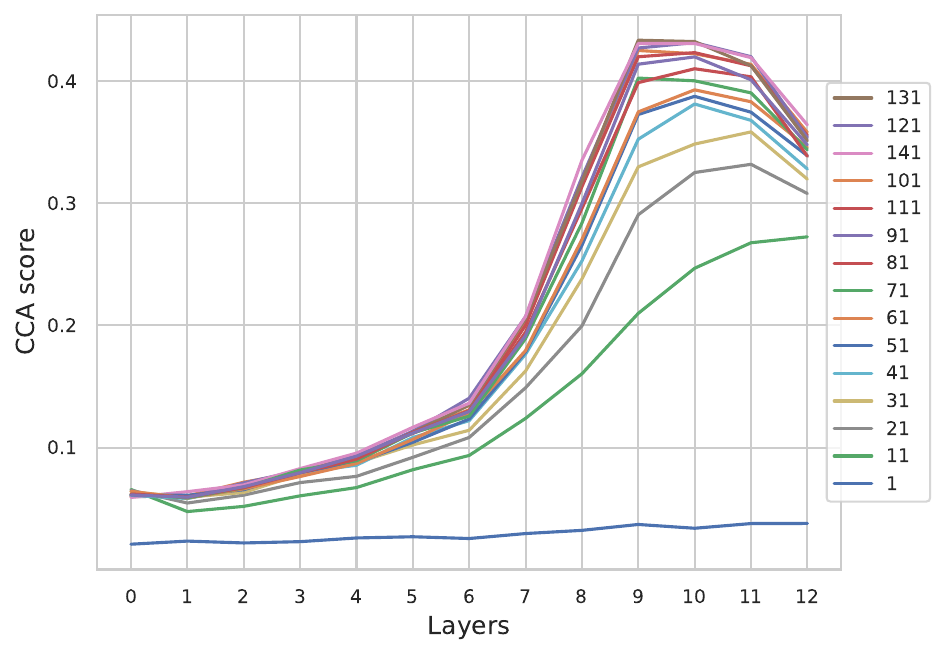}
        
    \end{minipage}
    \centering
    \begin{minipage}{0.32\linewidth}
        \caption*{\tiny{Wav2vec2.0 - Word} }
        \includegraphics[width=\textwidth]{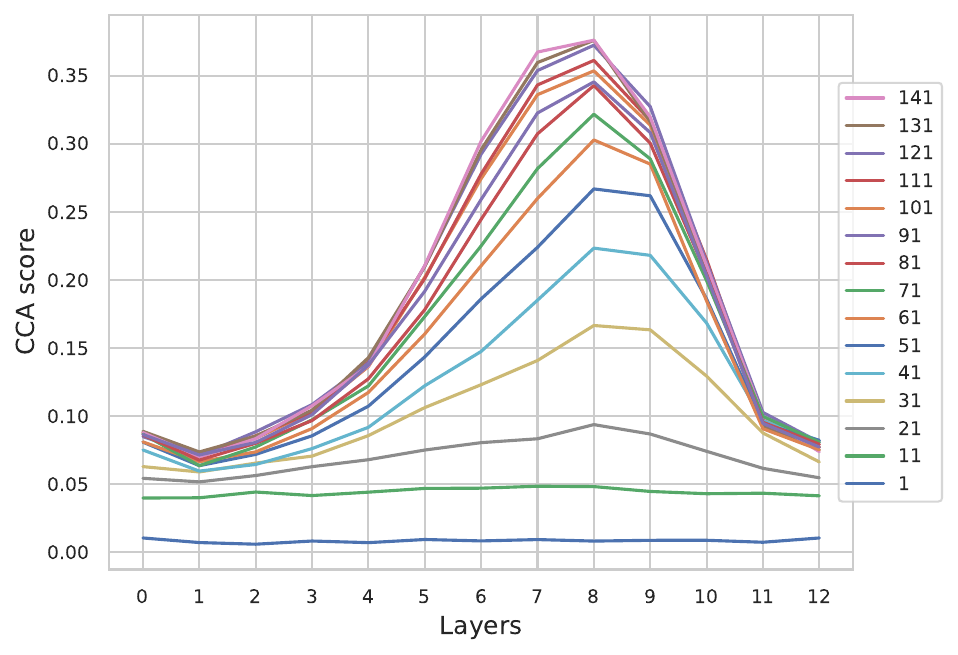}
        
    \end{minipage}
     \centering
    \begin{minipage}{0.32\linewidth}
        \caption*{\tiny{HuBERT First Iteration - Phone} }
        \includegraphics[width=\textwidth]{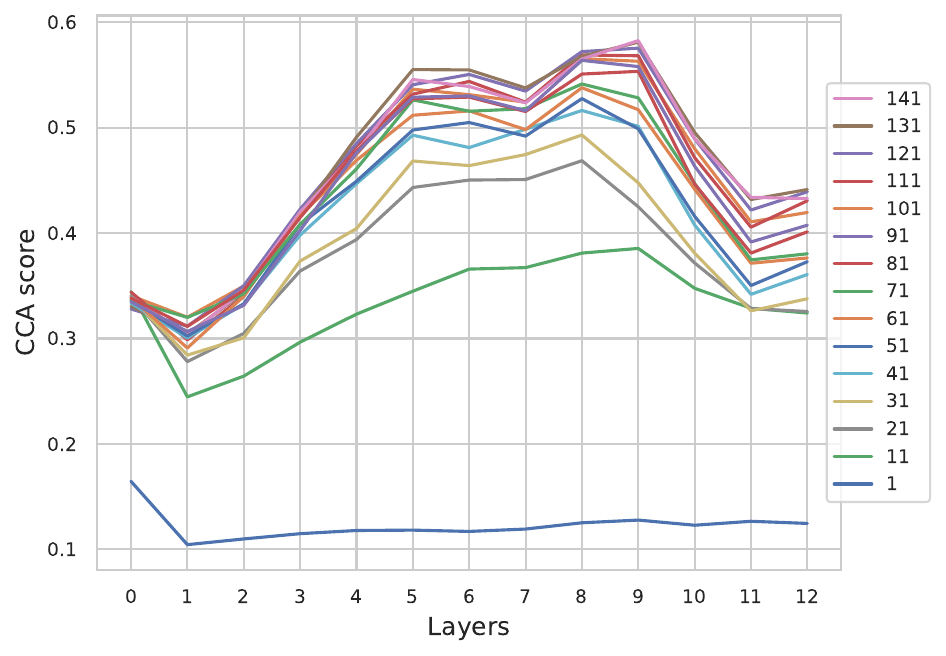} 
        
    \end{minipage}
    \centering
    \begin{minipage}{0.32\linewidth}
        \caption*{\tiny{HuBERT Second Iteration - Phone} }
        \includegraphics[width=\textwidth]{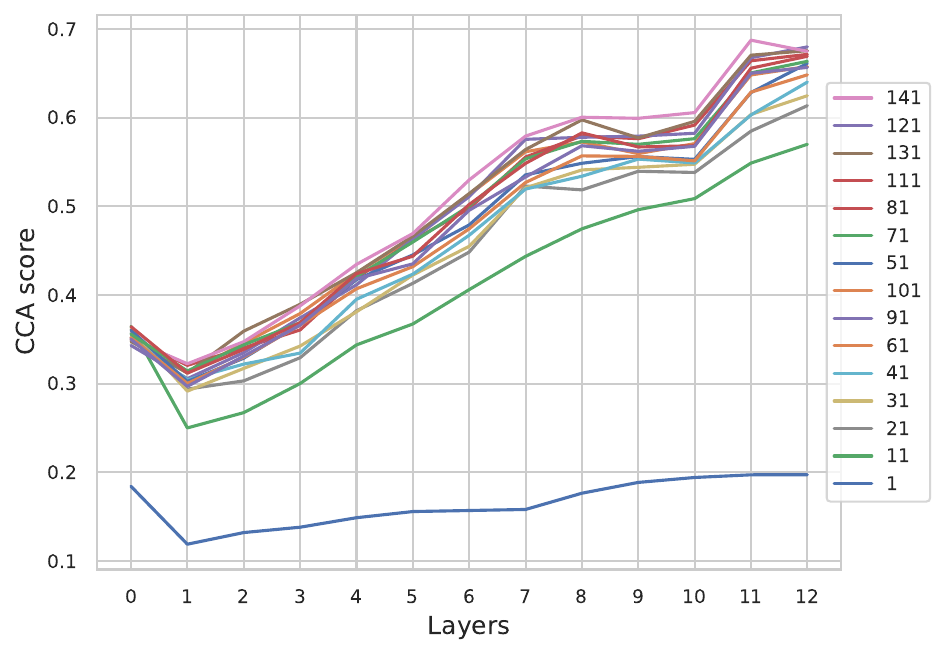}
        
    \end{minipage}
    \centering
    \begin{minipage}{0.32\linewidth}
        \caption*{\tiny{Wav2vec2.0 - Phone} }
        \includegraphics[width=\textwidth]{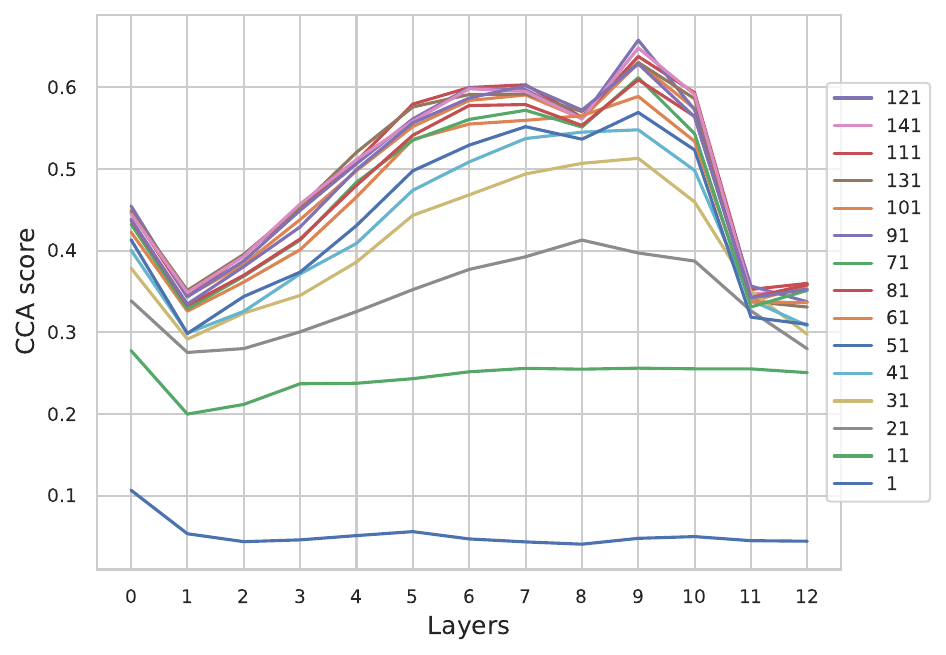}
        
    \end{minipage}
         \centering
    \begin{minipage}{0.32\linewidth}
        \caption*{\tiny{HuBERT First Iteration - Wrt Layer 0} }
        \includegraphics[width=\textwidth]{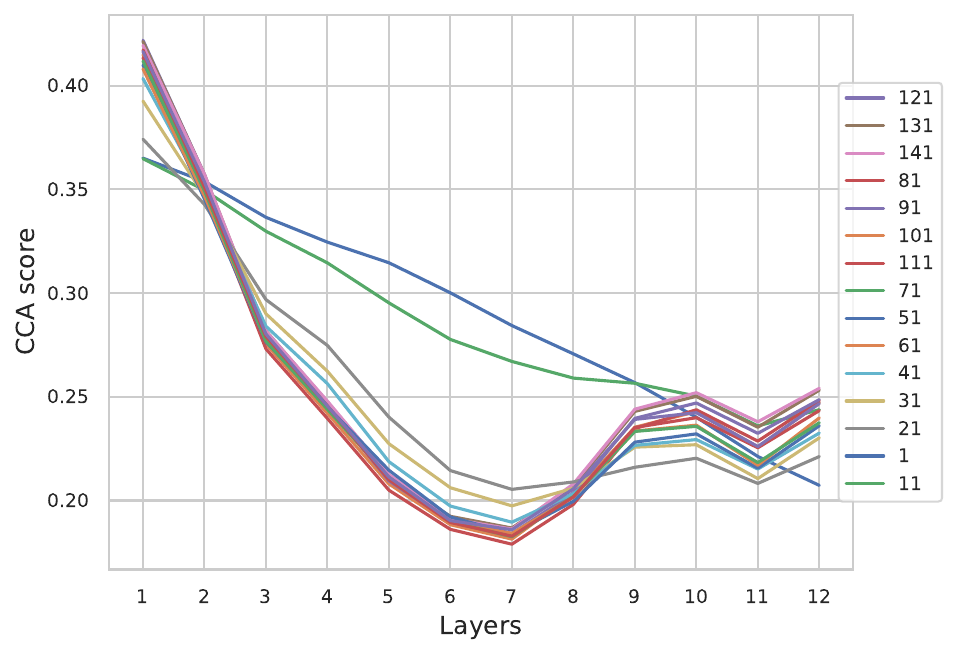} 
        
    \end{minipage}
    \centering
    \begin{minipage}{0.32\linewidth}
        \caption*{\tiny{HuBERT Second Iteration - Wrt Layer 0} }
        \includegraphics[width=\textwidth]{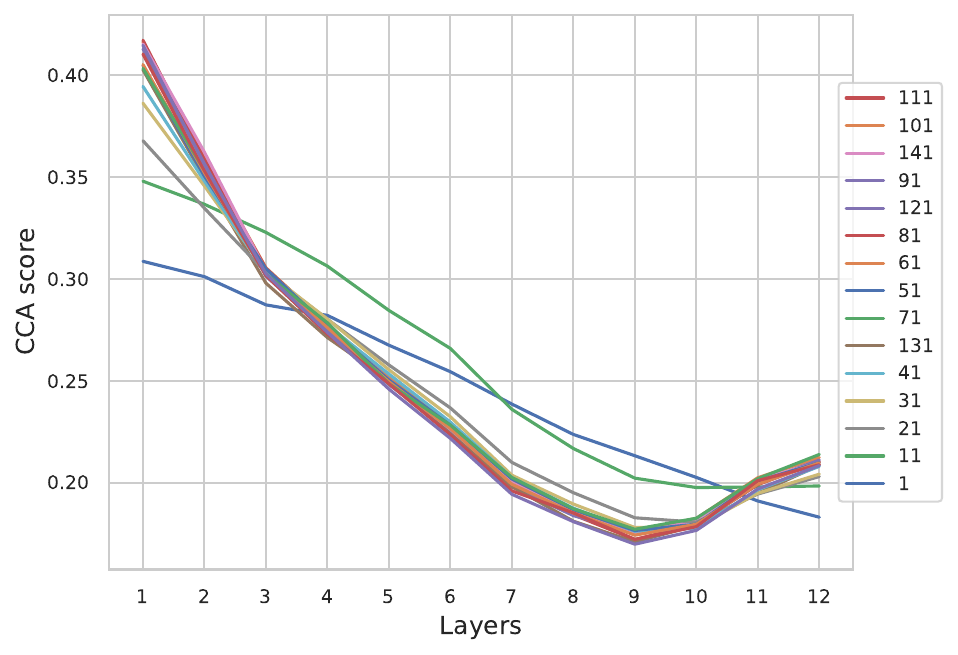}
        
    \end{minipage}
    \centering
    \begin{minipage}{0.32\linewidth}
        \caption*{\tiny{Wav2vec2.0 - Wrt Layer 0} }
        \includegraphics[width=\textwidth]{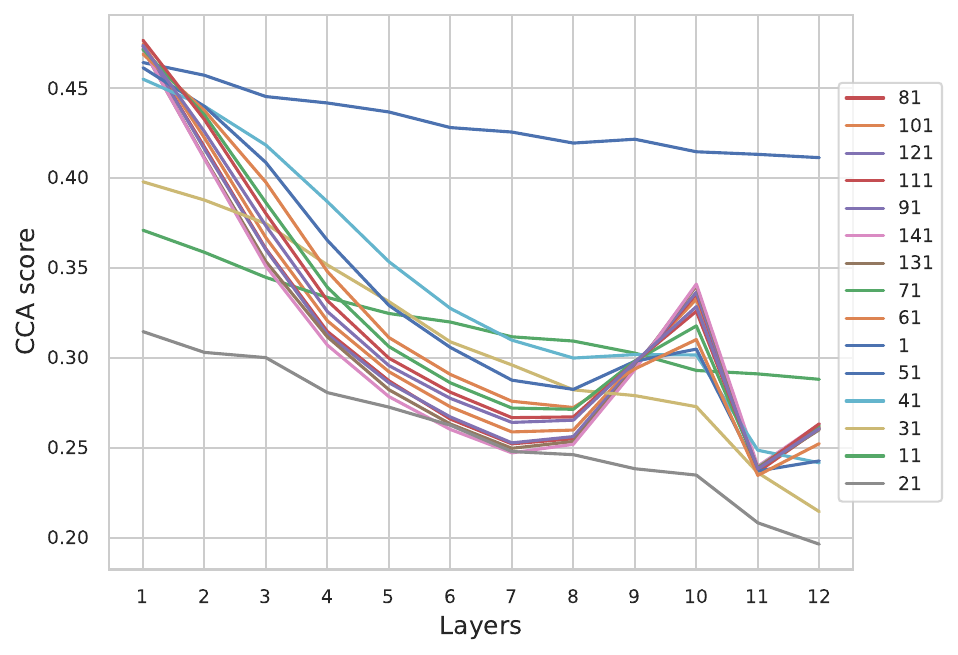}
        
    \end{minipage}
\caption{Different self-supervised speech approaches evaluated at various epochs of pretraining.}
\label{fig:all_layerwise}
\end{figure*}
